# Supplementary material for: INSCIT: Information-Seeking Conversations with Mixed-Initiative Interactions
Source: arXiv:2207.00746 source file (2023-06-22)
Supplement: Supplementary file 1 [file appendix.tex]

\newpage

\section{User and Agent Data Collection Interfaces}

\begin{figure}[h]
\centering
\includegraphics[width=1.0\linewidth]{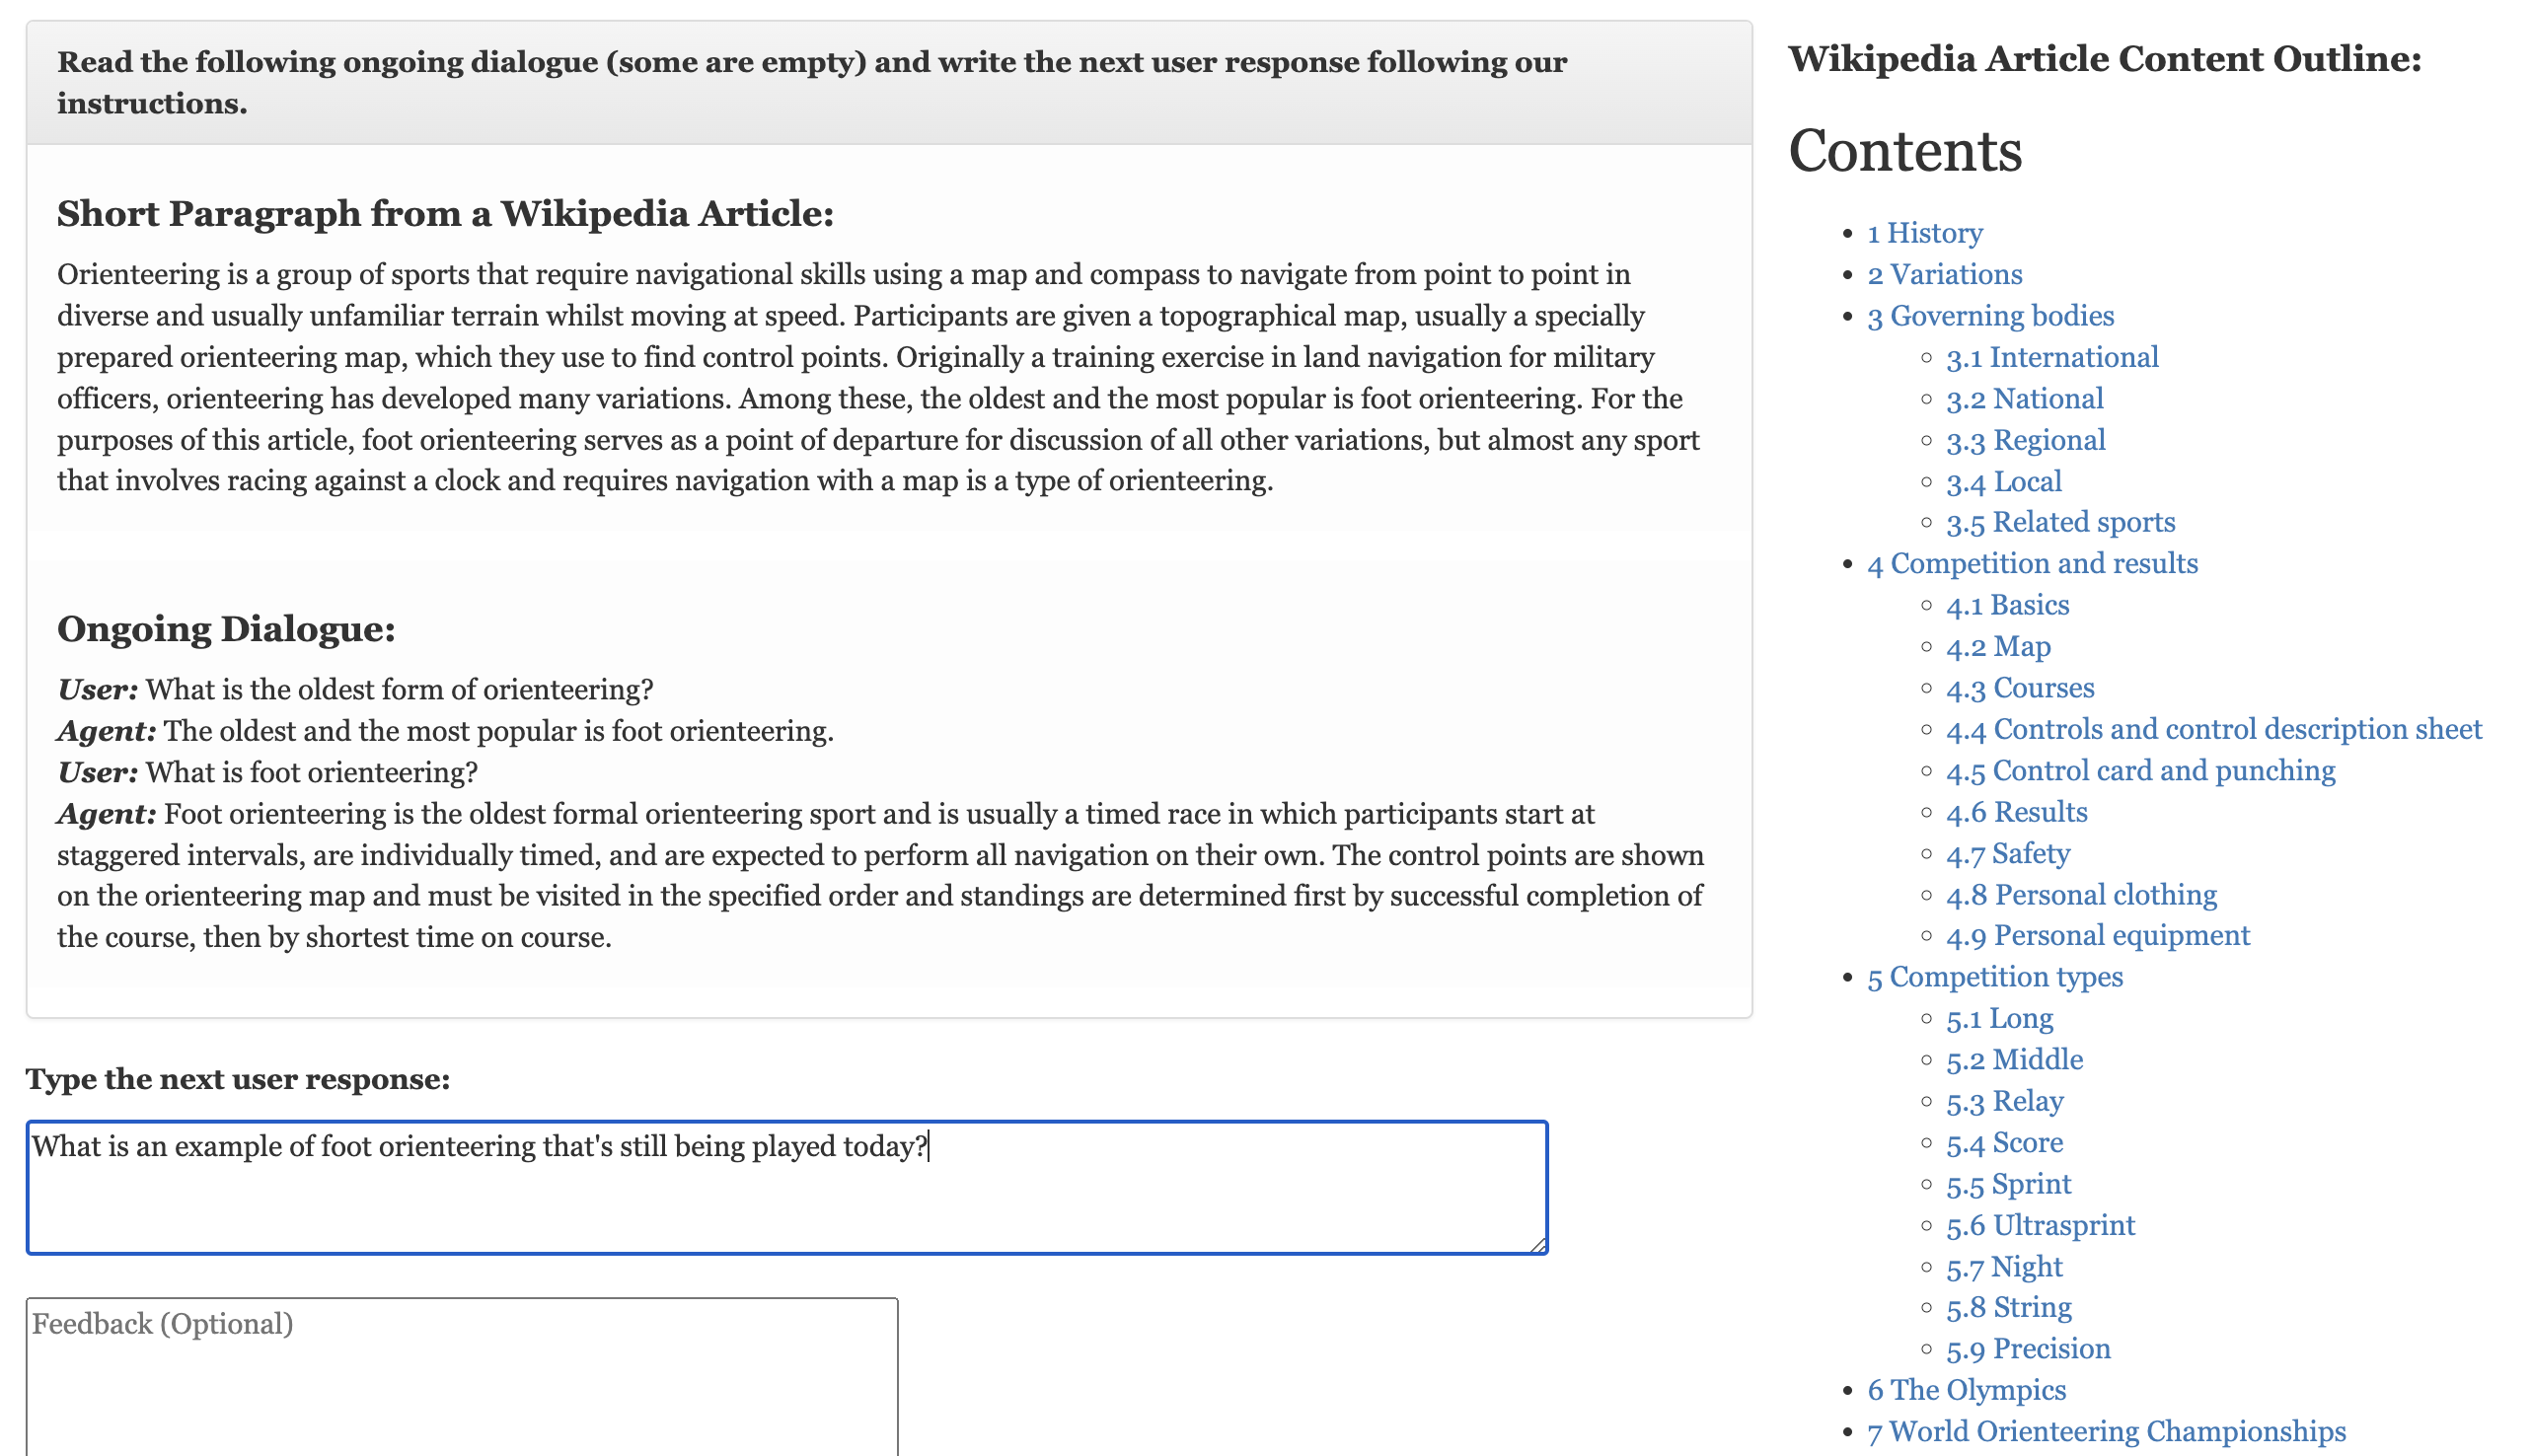}
\caption{\label{fig:user_interface} User annotation interface.}
\end{figure}

\begin{figure}[h]
\centering
\includegraphics[width=1.0\linewidth]{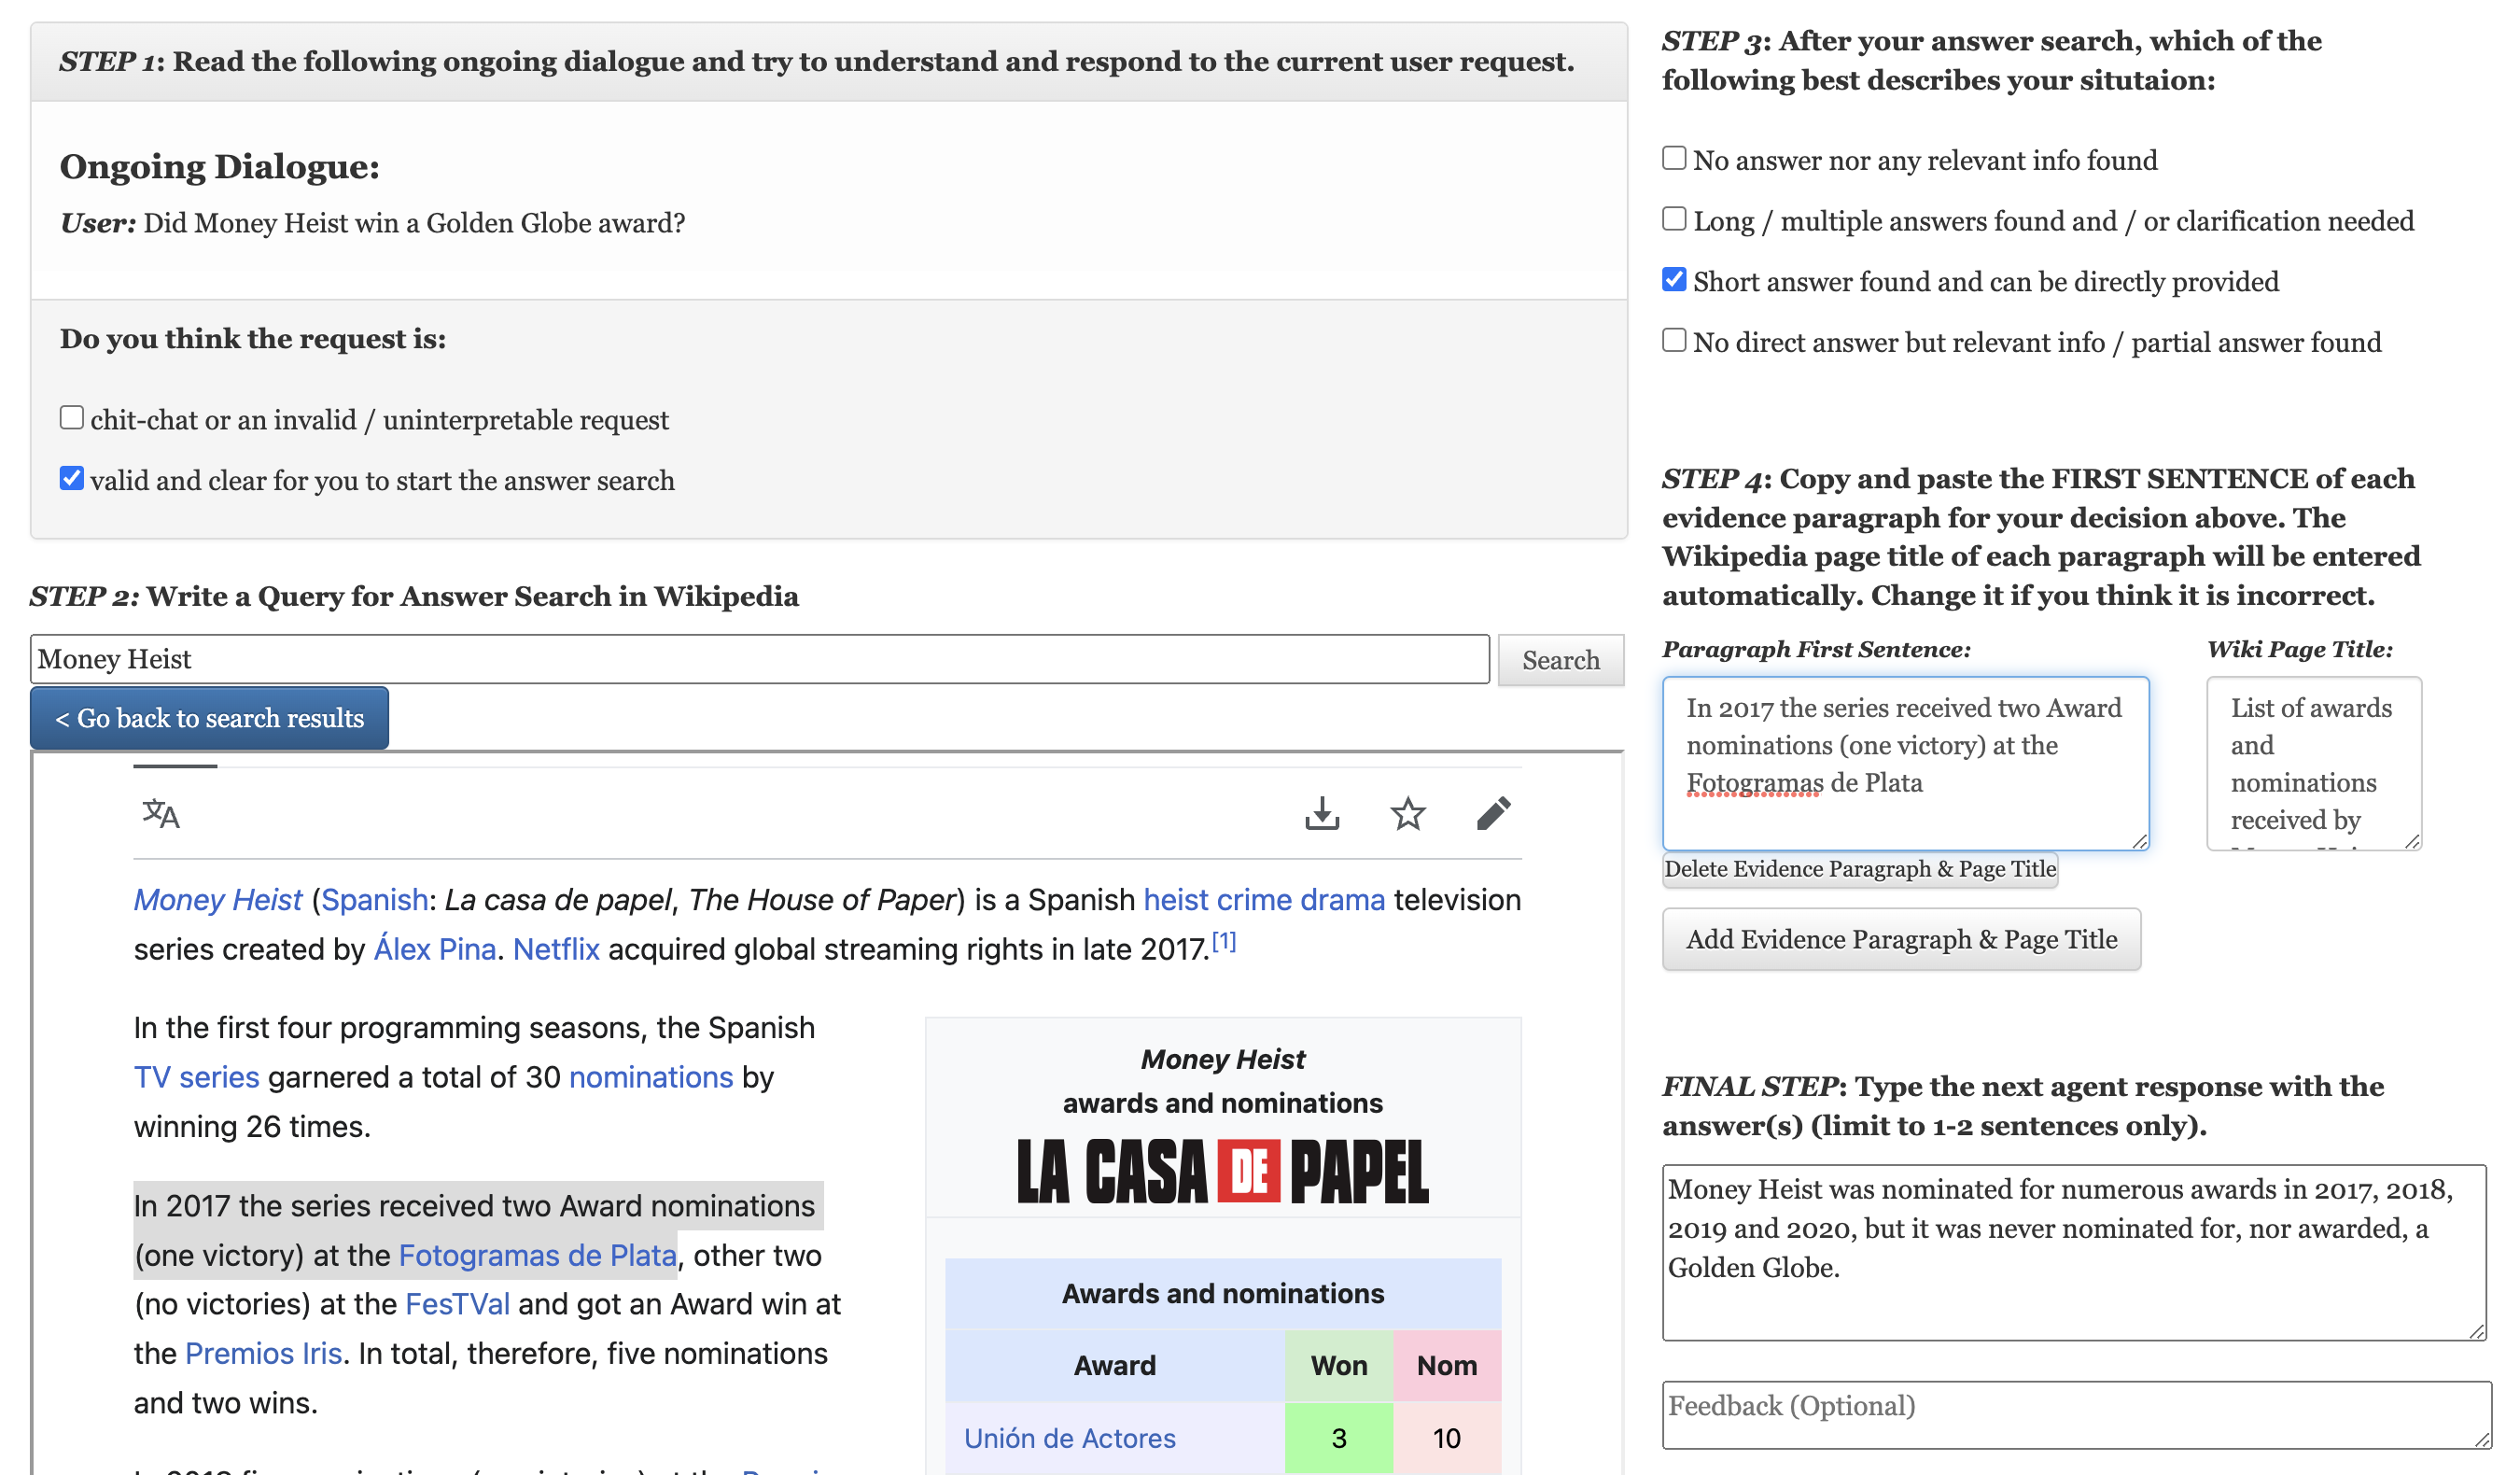}
\caption{\label{fig:agent_interface} Agent annotation interface.}
\end{figure}
